# Supplementary material for: Atomically Abrupt Topological p-n Junction
Source: arXiv:1708.07426 source file (2017-08-23)
Supplement: Supplementary file 1 [file Supporting_Information_for_Atomically_Abrupt_Topological_p-n_Junction.pdf]

*Supporting Information for*

# Atomically Abrupt Topological *p-n* Junction

Sung Hwan Kim,[1, 2] Kyung-Hwan Jin,[3] Byung Woo Kho,[2] Byeong-Gyu Park,[4] Feng Liu,[3,5] Jun Sung Kim,[2] and Han Woong Yeom[1, 2]

[1]*Center for Artificial Low Dimensional Electronic Systems, Institute for Basic Science, Pohang 37673, Republic of Korea*

[2]*Department of Physics, Pohang University of Science and Technology (POSTECH), Pohang 37673, Republic of Korea*

[3]*Department of Materials Science and Engineering, University of Utah, Salt Lake City, Utah 84112, USA*

[4]*Pohang Accelerator Laboratory, Pohang University of Science and Technology (POSTECH), Pohang 37673, Republic of Korea*

[5]*Collaborative Innovation Center of Quantum Matter, Beijing 100084, China*

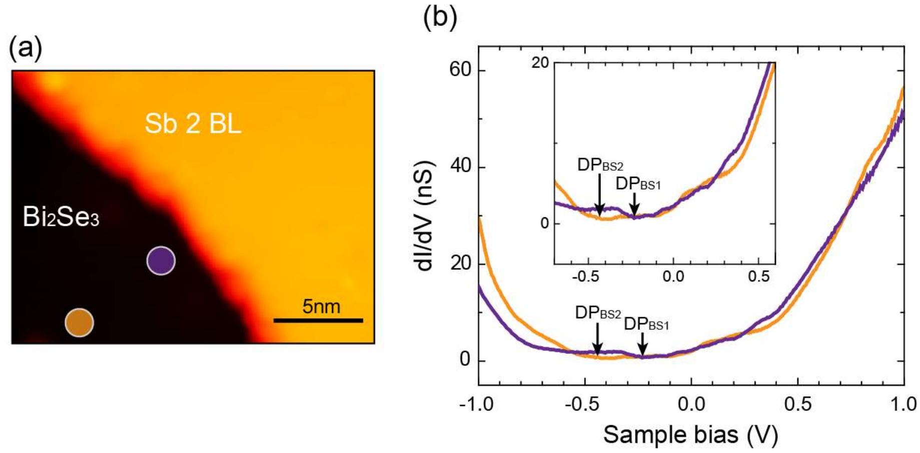


**Figure S1. STS measurements on a $Bi_2Se_3$ surface.** (a) STM topography images of Sb(2BL's)/$Bi_2Se_3$ [Fig. 5(a)]. (b) The *dI/dV* (STS) curves obtained from two points (violet and orange dots) on the $Bi_2Se_3$ surface, which are near (violet dot) and away (orange) from the edge of the Sb island, respectively. The violet and orange curves from the positions indicated by violet and orange dots of (a). The inset enlarges the spectra around the Dirac point of $Bi_2Se_3$, which is shifted closer to the Fermi energy due to the doping effect of Sb.

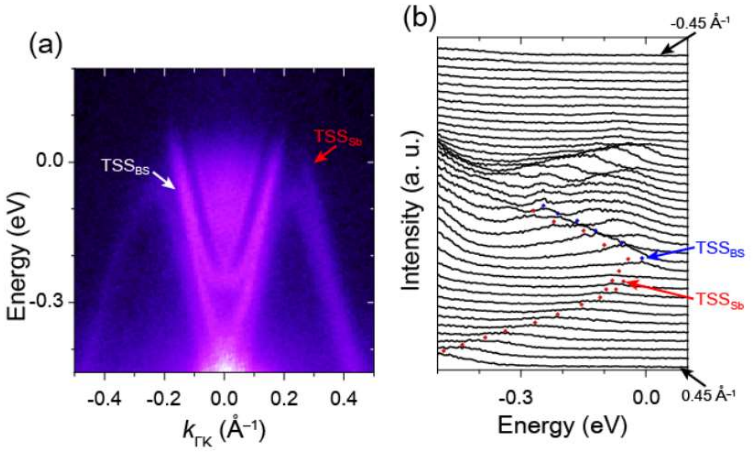


**Figure S2.** (a) High resolution ARPES measurement of Sb/$Bi_2Se_3$ [Fig. 3(a)]. (b) Energy distribution curves (EDC) extracted from (a). The red and blue dots in indicate the $TSS_{Sb}$ and $TSS_{BS}$, respectively.

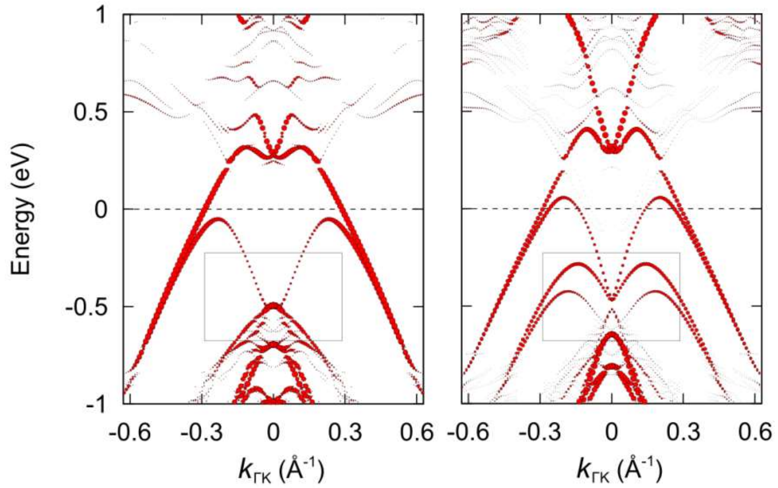


**Figure S3. Comparison of the band structures for 2 (right) and 3 (left) BL Sb/$Bi_2Se_3$.**

## Theoretical support of the mechanism for the formation of the p-type topological surface state by Sb layers:

To better understand the heterostructure of 2 BL Sb/$Bi_2Se_3$ system, we construct the effective model Hamiltonian[1-3]. The low-energy effective Hamiltonian for the topological surface state (TSS) of a topological insulator (TI) thin film can be written as,

$$H_{\text{eff}} = \begin{bmatrix} h_+(k) & 0 \\ 0 & h_-(k) \end{bmatrix},$$

with the basis $|\Psi\rangle = \left(|\Psi_t^{\uparrow}\rangle,\ |\Psi_t^{\downarrow}\rangle,\ |\Psi_b^{\uparrow}\rangle,\ |\Psi_b^{\downarrow}\rangle\right)$, where $|\Psi_{t(b)}^{\uparrow\downarrow}\rangle$ is the topological surface state for top (bottom) surface. The TI surface sates are described by a massless Dirac cone with helical spin texture,

$$h_+(k) = E_0 - Dk^2 + \begin{bmatrix} \Delta/2 - Bk^2 + Ck^4 & Ak_- \\ Ak_+ & -\Delta/2 + Bk^2 - Ck^4 \end{bmatrix},$$

$$h_-(k) = E_0 - Dk^2 + \begin{bmatrix} -\Delta/2 + Bk^2 - Ck^4 & -Ak_- \\ -Ak_+ & \Delta/2 - Bk^2 + Ck^4 \end{bmatrix},$$

where $k_\pm = k_x \pm ik_y$ and A, B, C, D and Δ are fitting parameters for TI thin films.

To describe the coupling between Sb 2BL and $Bi_2Se_3$ TSS's [Fig. S4(a)], we construct an expanded Hamiltonian,

$$H_{\mathrm{hetero}} = \begin{bmatrix} H_{\mathrm{eff}}^{\mathrm{Sb\,2BL}}(k) & T \\ T^\dagger & H_{\mathrm{eff}}^{\mathrm{Bi_2Se_3}}(k) \end{bmatrix}.$$

The surface states of Sb 2BL, $H_{\mathrm{eff}}^{\mathrm{Sb\,2BL}}$, is written as

$$H_{\mathrm{eff}}^{\mathrm{Sb\,2BL}}(k) = H_{\mathrm{eff}}(k) + \begin{bmatrix} \delta 1_{2\times 2} & 0 \\ 0 & 0 \end{bmatrix},$$

where the parameter δ describes potential difference between top and bottom surfaces of Sb 2BL due to the charge transfer in the heterostructure. The hopping between the bottom TSS of 2 BL Sb and the top TSS of $Bi_2Se_3$ is given as

$$T = \begin{bmatrix} 0 & 0 \\ t\sigma_z & 0 \end{bmatrix},$$

with the parameter *t* characterizing the interfacial coupling of the heterostructure. Note, they have opposite helicity to allow the coupling between them.

Figure S4(b) and S4(c) show the TSS's of the effective model for pristine Sb 2BL and $Bi_2Se_3$, respectively. Table S1 shows the fitting parameter which we used for the pristine Sb 2BL and $Bi_2Se_3$ surface states. For the Sb 2BL, there is coupling between top and bottom TSS'ss and the gap is opened at the Dirac point.

For the TSS'ss of $Bi_2Se_3$, we considered the electron-doped TSS'ss to match with the experimental result. Figure S2(d) show the band structure of model Hamiltonian for the 2 BL Sb /Bi2Se3 heterostructure. Immediate changes when the interaction between bottom TSS of 2 BL Sb and TSS $Bi_2Se_3$ is included are the hybridization gap which is proportional to parameter *t* and a shift in Dirac point of $Bi_2Se_3$. The Dirac points of bottom TSS of Sb 2BL and $Bi_2Se_3$ are still preserved but the

hybridization gap is opened near the Fermi level. The both side of TSSs are destroyed by this interfacial interaction. While the other top TSS of Sb 2BL replaces the original TSSs of $Bi_2Se_3$ [shaded area in Fig. S2(d)]. The Dirac point of the top TSS of Sb 2BL is recovered due to the vanished coupling interaction between top and bottom TSS's. But the Dirac point shifts to higher energy and forms hole-doped Dirac states due to the charge transfer from Sb to the $Bi_2Se_3$ top surface. We calculated the charge transfer using Bader analysis[4] and found that 0.14e have been transferred from Sb 2BL. The Sb layer acts as a donor and the $Bi_2Se_3$ as an acceptor, with the electrons transferring from the former to the latter. The hole type TSS of the top Sb layer is controlled by the parameter δ and here we set δ=0.25 eV.

| Film | $E_0$ (eV) | D (eV Å$^2$) | Δ (eV) | C (eV Å$^4$) | B (eV Å$^2$) | A ($10^5$ ms$^{-1}$) |
|---|---|---|---|---|---|---|
| **Sb 2BL** | –0.1 | –78.08 | 0.152 | –461.44 | 66.56 | 3.104 |
| **$Bi_2Se_3$** | –0.214 | –13 | 0 | 0 | 9.0 | 4.28 |

**Table S1**. The fitting parameters for the Sb 2BL and $Bi_2Se_3$ thin films.

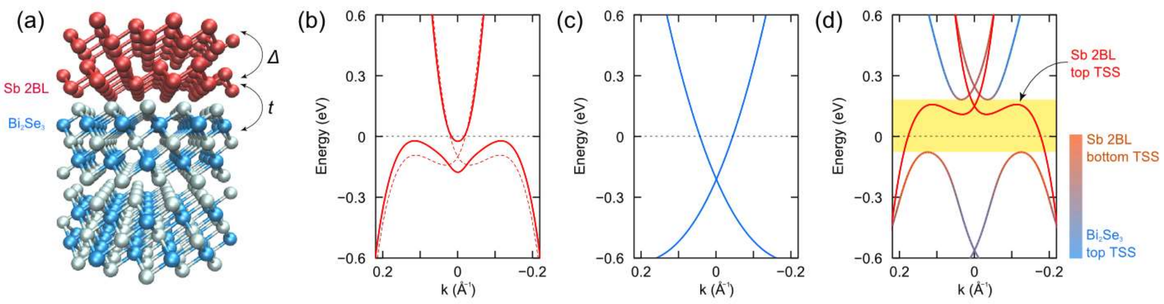


**Figure S4** (a) Heterostructure of 2 BL Sb/$Bi_2Se_3$. The coupling between bottom TSS of 2 BL Sb and top TSS of $Bi_2Se_3$ controlled by parameter *t*. (b) Effective model band structure of pristine Sb 2 BL. The gap is opened due to coupling between top and bottom TSS of 2 BL Sb which is proportional to Δ. (c) Effective model band structure for the electron-doped TSS of pristine $Bi_2Se_3$. (d) Band structure of Sb 2BL/$Bi_2Se_3$ with coupling parameter *t*=0.4 eV. The hybridization gap is opened (yellow shade) between bottom TSS of 2 BL Sb and top TSS of $Bi_2Se_3$. The bottom TSSs of $Bi_2Se_3$ is not shown here.

This picture of 3D TI/TI heterostructures is quite general and we further studied using simple 3D TIs [Fig. S5]. We construct 1 QL TI/5QL TI heterostructure, such as 1 QL $Bi_2Te_3$ on 5 QL $Bi_2Se_3$ thin films and vice versa [Fig. S5(a) and S5(b)]. The covered 1QL TI thin film has a gap due to the coupling between top and bottom surfaces. Calculated band structure for the pristine 6QL $Bi_2Se_3$ and $Bi_2Te_3$ thin films and 1 QL/5 QL TI heterostructures shown in Fig. S5(c) and S5(d). Compared with the pristine 6 QL $Bi_2Se_3$ and $Bi_2Te_3$ thin film, the Dirac states of the heterostructures still exist and are mainly contributed by a covered 1 QL TI thin film[5,6]. The topological surface states are totally replaced by covered 1 QL TI thin film. These results suggest that the 3D TI/TI heterostructure didn't change the bulk band nontrivial $Z_2$ topology, while it can modify the topological surface state. These results are consistent with our effective model and 2 BL Sb/$Bi_2Se_3$ heterostructure.

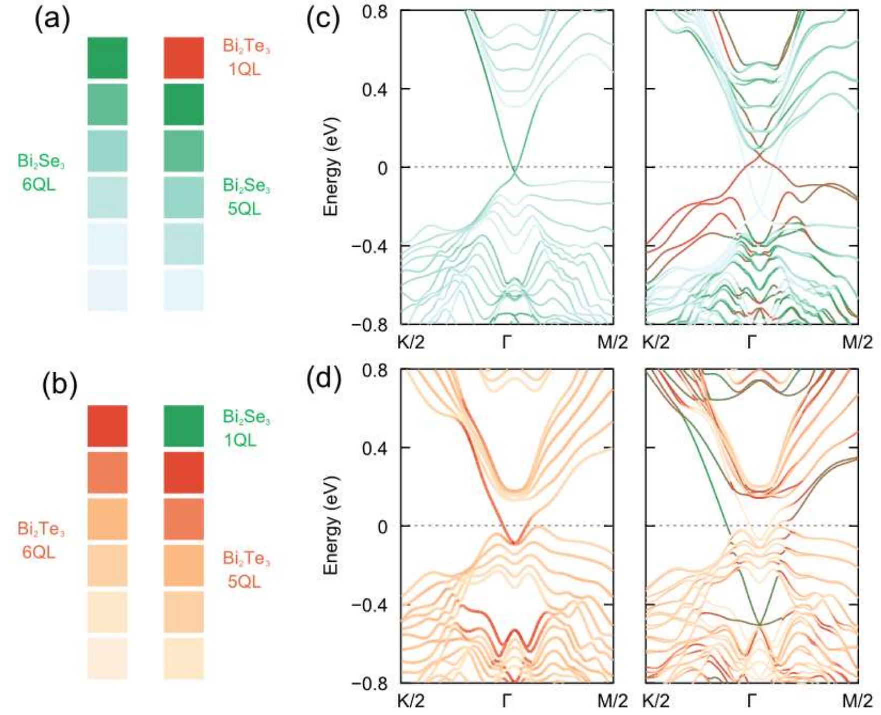


**Figure S5** (a), (b) Schematic pristine- and hetero-3D TI slab structures using $Bi_2Se_3$ and $Bi_2Te_3$. The slab structure is composed with 1 QL TI/5QL TI heterostructure, such as 1 QL $Bi_2Te_3$ on 5 QL $Bi_2Se_3$ thin films and vice versa. (c), (d) Calculated surface band structures for pristine and hetero slab structure in (a) and (b), respectively. The color indicates the bands induced by each QLs in (a) and (b).

## References


1. Shan, W.-Y.; Lu, H.-Z.; Shen, S.-Q. Effective Continuous Model for Surface States and Thin Films of Three-Dimensional Topological Insulators. *New J. Phys.* **2010**, 12, 043048.

*2.* Lu, H.-Z.; Shan, W.-Y.; Yao, W.; Niu, Q.; Shen, S.-Q. Massive Dirac Fermions and Spin Physics in an Ultrathin Film of Topological Insulator. *Phys. Rev. B: Condens. Matter Mater. Phys,* **2010**, 81, 115407.

3. Jin, K.-H.; Yeom, H.W.; Jhi, S.-H. Band Structure Engineering of Topological Insulator Heterojunctions. *Phys. Rev. B: Condens. Matter Mater. Phys* **2016**, 93, 075308.

4. Henkelman, G.; Arnaldsson, A.; Jónsson, H. A Fast and Robust Algorithm for Bader Decomposition of Charge Density. *Comp. Mat. Sci.* **2006**, 36, 354–360.

5. Zhao, Y.; Chang, C.-Z.; Jiang, Y.; DaSilva, A.; Sun, Y.; Wang, H.; Xing, Y.; Wang, Y.; He, K.; Ma, X.; Xue, Q.-K.; Wang. J. Demonstration of Surface Transport in a Hybrid $Bi_2Se_3$/$Bi_2Te_3$ Heterostructure. *Sci. Rep.* **2013**, 3, 3060.

6. Chang, C.-Z.; Tang, P.; Feng, X.; Li, K.; Ma, X.-C.; Duan, W.; He, K.; Xue, Q.-K. Band Engineering of Dirac Surface States in Topological-Insulator-Based van der Waals Heterostructures. *Phys. Rev. Lett.* **2015**, 115, 136801
